# Supplementary material for: mvn2vec: Preservation and Collaboration in Multi-View Network Embedding
Source: arXiv:1801.06597 source file (2019-11-03)
Supplement: Supplementary file 1 [file appendix.tex]

%!TEX root = mvn2vec.tex

\section*{Appendix}
We provide the gradients used for ASGD in the proposed algorithms.

\vpara{\mtvcon}:
%\begin{footnotesize}
\begin{small}
\begin{align}\label{eq::mtv-con-grad-1}
\frac{\partial \mc{O}_{\textsc{con}}}{\partial \mbf^v_u} = & \left( 1 - \sigma(\mbf^v_u \cdot \funcphi{n}) \right) \cdot \funcphi{n} \nonumber \\ %[-4pt]
- & \sum_{i=1}^K \sigma(\mbf^v_u \cdot \funcphi{n'_i}) \cdot \funcphi{n'_i},
\end{align}
%%\vspace{-6pt}
\begin{equation}\label{eq::mtv-con-grad-2}
\frac{\partial \mc{O}_{\textsc{con}}}{\partial \tilde\mbg^{\hat{v}}_n} =  \left( 1 - \sigma(\mbf^v_u \cdot \funcphi{n}) \right) \cdot \mbf^v_u \cdot
\begin{cases}
\theta + \frac{1 - \theta}{|\mc{V}|},\; & \hat{v} = v,\\
\theta, \; & \hat{v} \neq v,
\end{cases} 
\end{equation}
%%\vspace{-3pt}
\begin{equation}\label{eq::mtv-con-grad-3}
\frac{\partial \mc{O}_{\textsc{con}}}{\partial \tilde\mbg^{\hat{v}}_{n'_i}} = - \sigma(\mbf^v_u \cdot \funcphi{n'_i}) \cdot \mbf^v_u \cdot
\begin{cases}
\theta + \frac{1 - \theta}{|\mc{V}|},\; & \hat{v} = v,\\
\theta, \; & \hat{v} \neq v.
\end{cases}
\end{equation}
\end{small}
%%\vspace{-6pt}

\vpara{\mtvreg}:
\begin{small}
\begin{align}\label{eq::mtv-reg-grad-1}
\frac{\partial \mc{O}_{\textsc{reg}}}{\partial \mbf^v_u} = & \left( 1 - \sigma(\mbf^v_u \cdot  \tilde{\mbf}^v_n) \right) \cdot \tilde{\mbf}^v_n - \sum_{i=1}^K  \sigma(\mbf^v_u \cdot  \tilde{\mbf}^v_{n'_i}) \cdot  \tilde{\mbf}^v_{n'_i}    \nonumber \\ %[-3pt]
+ & 2  \gamma  \Big(K+1\Big)  \Big(1-\frac{1}{|\mc{V}|}\Big) \cdot \Big(\mbf^v_{{u}} - \frac{1}{|\mc{V}|} \sum_{v' \in \mc{V}} \mbf^{v'}_{{u}}\Big), 
\end{align}
%%\vspace{-6pt}
\begin{align}\label{eq::mtv-reg-grad-2}
\frac{\partial \mc{O}_{\textsc{reg}}}{\partial \tilde\mbf^{{v}}_n} = &  \left( 1 - \sigma(\mbf^v_u \cdot \tilde\mbf^{{v}}_n) \right) \cdot \mbf^v_u 
+ 2  \gamma  \Big(1-\frac{1}{|\mc{V}|}\Big) \cdot \Big(\tilde\mbf^v_{n} - \frac{1}{|\mc{V}|} \sum_{v' \in \mc{V}} \tilde\mbf^{v'}_{n}\Big),
\end{align}
%%\vspace{-6pt}
\begin{align}\label{eq::mtv-reg-grad-3}
\frac{\partial \mc{O}_{\textsc{reg}}}{\partial \tilde\mbf^{{v}}_{n'_i}} = & - \sigma(\mbf^v_u \cdot \tilde\mbf^{{v}}_{n'_i}) \cdot \mbf^v_u 
+ 2  \gamma  \Big(1-\frac{1}{|\mc{V}|}\Big) \cdot \Big(\tilde\mbf^v_{n'_i} - \frac{1}{|\mc{V}|} \sum_{v' \in \mc{V}} \tilde\mbf^{v'}_{n'_i}\Big).
\end{align}
\end{small}
%%\vspace{-6pt}

Note that in implementation, $|V|$ should be the number of views in which $u$ is associated with at least one edge.
